# Supplementary material for: Self-Supervised Path Planning in Unstructured Environments via Global-Guided Differentiable Hard Constraint Projection
Source: arXiv:2601.19354 source file (2026-01-27)
Supplement: Supplementary file 1 [file Supplement.pdf]

# Supplementary Material
# Self-Supervised Path Planning in Unstructured Environments via Global-Guided Differentiable Hard Constraint Projection

Ziqian Wang[1,2], Chenxi Fang[3] and Zhen Zhang[*,1,2]

[1]State Key Laboratory of Tribology in Advanced Equipment, Tsinghua University, Beijing 100084, China
[2]Beijing Key Laboratory of Transformative High-end Manufacturing Equipment and Technology, Department of Mechanical Engineering, Tsinghua University, Beijing 100084, China
[3]Automotive Electronics Business Unit at Hirain Inc., China
[*]To whom correspondence should be addressed. E-mail: zzhang@tsinghua.edu.cn (Zhen Zhang)

## Contents

**S1 Visualization of LSE-based obstacle representation 1**

**S2 Testing Scenario Generation 1**

**S3 Implementation details of baseline methods 3**
S3.1 Hybrid A* . . . . . . . . . . . . . . . . . . . . . . . . . . . . . . . . 3
S3.2 Informed RRT* . . . . . . . . . . . . . . . . . . . . . . . . . . . . . 3
S3.3 NMPC . . . . . . . . . . . . . . . . . . . . . . . . . . . . . . . . . . 4

**S4 Implementation details of Carla simulation 4**

## S1 Visualization of LSE-based obstacle representation

This section visualizes the smooth collision constraint field generated by the Log-Sum-Exponential (LSE) operator. As illustrated in Fig. S1, the blue solid lines represent the zero-isocontour $C_{\text{obs}}(\mathbf{p}) = 0$, denoting the approximated obstacle boundaries. With the selected $\alpha = 10$, the representation maintains high geometric fidelity to the original quadrilaterals while ensuring a smooth gradient landscape for stable optimization.

## S2 Testing Scenario Generation

The ego vehicle is initialized at a fixed start configuration $\mathbf{p}_{start} = [0, 0]^T$ with an initial heading along the positive $x$-axis ($\theta_0 = 0°$).

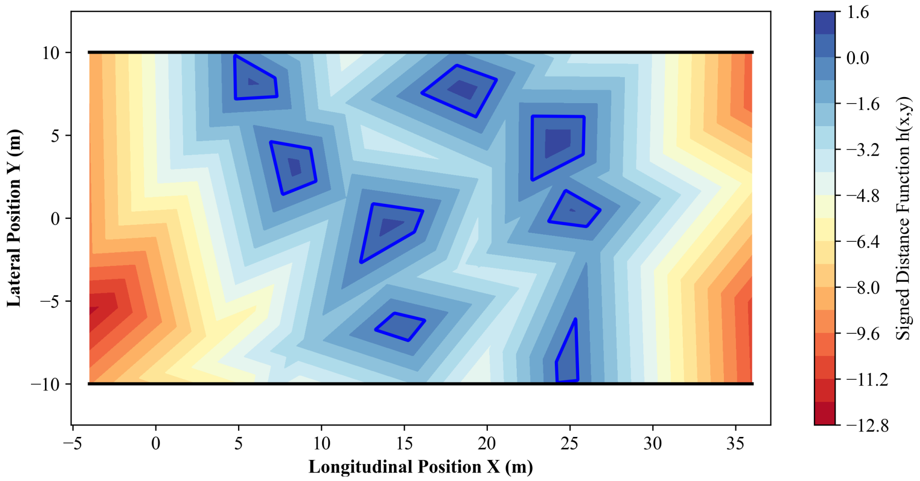


Figure S1: Visualization of LSE-based obstacle representation. The blue solid lines indicate the zero-isocontour $C_{\text{obs}}(\mathbf{p}) = 0$, approximating the obstacle boundaries. The smooth gradient field facilitates effective collision avoidance in optimization.

The environment layout is spatially partitioned into an obstacle generation zone and a goal sampling zone. Obstacles are spawned within the region $x \in [4, 28]$ m and $y \in [-10, 10]$ m, while goal points are sampled from the region $x \in [30, 34]$ m and $y \in [-8, 8]$ m.

For each scenario, we generate $N_{obs} = 8$ random quadrilateral obstacles. The geometry of each obstacle is randomized, with side lengths sampled from a uniform distribution $l \sim \mathcal{U}(1, 4)$ meters (see Fig. S2). To ensure the existence of feasible topological channels for a vehicle with a width of 2.0 m, we enforce a strict minimum clearance constraint: during generation, any new obstacle must maintain a distance of at least 2.5 m from existing obstacles.

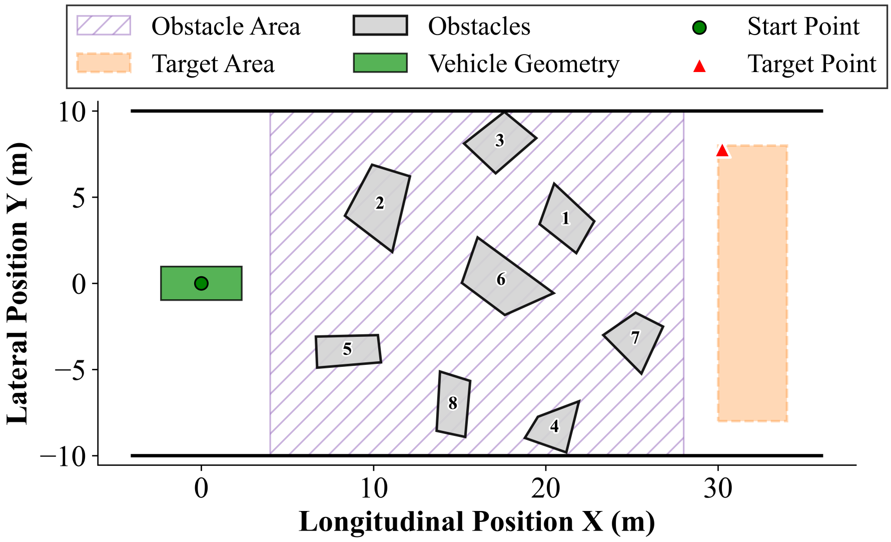


Figure S2: Example of a generated unstructured environment with randomly placed obstacles (gray polygons), the ego vehicle's start position (green square), and the goal region (red triangle). Obstacles are generated within the purple area, while goals are sampled in the orange area.

## S3 Implementation details of baseline methods

### S3.1 Hybrid A*

The Hybrid A* algorithm is implemented based on the open-source code from `https://github.com/AtsushiSakai/PythonRobotics.git`[S1].

The path planning module employs the Hybrid A* algorithm to search for kinematically feasible trajectories within a discretized configuration space $(x, y, \theta)$. The search tree is expanded using motion primitives generated by a discrete set of steering inputs. To enhance computational efficiency and convergence, an analytic expansion based on Reeds-Shepp curves is attempted whenever the vehicle approaches the goal region (distance $< 5.0\,\text{m}$) or at a fixed iteration frequency. The total cost function $f(n) = g(n)+h(n)$ integrates the accumulated path cost $g(n)$ and a heuristic cost $h(n)$ derived from a 2D dynamic programming map of holonomic obstacle distances. The accumulated cost $g(n)$ explicitly penalizes path length, direction switching (gear changes), reverse motion, steering effort, and rapid changes in steering angle to ensure trajectory smoothness. Obstacles are modeled as polygons with safety inflation, and collision checking is accelerated using a KD-Tree structure on discretized obstacle boundaries. The specific hyperparameters used in the algorithm are listed in Table S1.

Table S1: Hyperparameters for the Hybrid A* Planner

| **Parameter** | **Value** | **Parameter** | **Value** |
|---|---|---|---|
| XY Grid Resolution | 0.5 m | Switch Back Cost | 100.0 |
| Yaw Grid Resolution | 15.0° | Backward Cost | 5.0 |
| Motion Resolution | 0.1 m | Steer Change Cost | 5.0 |
| Steering Discrete Count | 5 | Steer Cost | 1.0 |
| Analytic Expansion Dist | 5.0 m | Heuristic Cost Weight | 5.0 |
| Analytic Expansion Freq | 10 | | |

### S3.2 Informed RRT*

The Informed RRT* algorithm is also implemented based on the open-source code from `https://github.com/AtsushiSakai/PythonRobotics.git`[S1]. The specific hyperparameters used in our implementation are detailed in Table S2.

Table S2: Hyperparameters for Informed RRT* Planner

| **Parameter** | **Value** | **Parameter** | **Value** |
|---|---|---|---|
| Expansion Step Size | 0.5 m | Obstacle Inflation | 1.2 m |
| Goal Sampling Rate | 10% | Rewiring Constant ($\gamma$) | 50.0 |
| Max Iterations | 1000 | Path Interp. Res. | 1.0 m |

### S3.3 NMPC

The NMPC problem is implemented using the CasADi framework and solved via the IPOPT interior-point solver. The optimization horizon is discretized into $T = 40$ steps with a sampling time of $\Delta t = 0.5\,\text{s}$. The objective function $J$ is formulated to minimize the deviation from the target state while penalizing control efforts and enforcing trajectory smoothness:

$$J = w_g \|p_T - p_{ref}\|^2 + \sum_{k=0}^{T-1} \left( w_u(v_k^2 + \delta_k^2) + w_s((\Delta v_k)^2 + (\Delta \delta_k)^2) \right) \tag{S1}$$

where $p_T$ is the terminal position, $u_k = [v_k, \delta_k]^T$ are the control inputs (velocity and steering angle), and $\Delta u_k$ represents the rate of change in controls. The optimization is subject to the kinematic bicycle model constraints, actuator limits, and the differentiable collision avoidance constraints described in the main text. To improve convergence, the solver is warm-started with a linear interpolation between the start and goal configurations.

Table S3: Hyperparameters for NMPC Planner

| **Parameter** | **Value** | **Parameter** | **Value** |
|---|---|---|---|
| Prediction Horizon ($T$) | 40 | Goal Weight ($w_g$) | 50.0 |
| Time Step ($dt$) | 0.5 s | Smoothness Weight ($w_s$) | 100.0 |
| Max Velocity | 5.0 m/s | Input Weight ($w_u$) | 1.0 |
| Max Steering | 40° | Max Acceleration | 2.0 m/$s^2$ |
| Safety Margin | 0.25 m | | |

## S4 Implementation details of Carla simulation

Table S4: Parameters for CARLA Simulation and Control

| **Parameter** | **Value** | **Parameter** | **Value** |
|---|---|---|---|
| Time Step ($\Delta t$) | 0.02 s | Lateral PID $K_P$ | 3.5 |
| Max Steering Angle | 40.0° | Lateral PID $K_I$ | 0.0 |
| Max Speed | 18.0 km/h | Lateral PID $K_D$ | 0.9 |
| Min Speed | 5.0 km/h | Long. PID $K_P$ | 0.8 |
| Max Lat. Accel. | 2.5 m/s$^2$ | Long. PID $K_I$ | 0.0 |
| Wheelbase | 2.87 m | Long. PID $K_D$ | 0.2 |

The experiments are conducted in the CARLA simulator using a flat asphalt environment. The simulation operates in *Synchronous Mode* with a fixed time step of $\Delta t = 0.02\,\text{s}$ (50 Hz) to ensure deterministic physics updates. The ego vehicle is based on the `vehicle.tesla.model3` blueprint, with the front-wheel maximum steering angle customized to 40°.

Trajectory tracking is executed by a coupled feedforward-feedback controller. Longitudinal control utilizes a PID regulator to track a dynamic reference speed $v_{cmd}$ derived from the local path curvature $\kappa$. This target speed is computed as

$$v_{cmd} = \text{clip}\left(\sqrt{\frac{a_{lat,max}}{|\kappa| + \epsilon}}, v_{min}, v_{max}\right)$$

, where $a_{lat,max} = 2.5\,\text{m/s}^2$ limits the lateral acceleration. For lateral control, the steering command integrates a PID feedback term with a geometric feedforward term $\delta_{ff} = \arctan(L \cdot \kappa)$, calculated using the kinematic bicycle model where $L$ is the wheelbase.

## References


[S1] Atsushi Sakai, Daniel Ingram, Joseph Dinius, Karan Chawla, Antonin Raffin, and Alexis Paques. Pythonrobotics: a python code collection of robotics algorithms. *arXiv preprint arXiv:1808.10703*, 2018.
